# Supplementary material for: All You Need is RAW: Defending Against Adversarial Attacks with Camera Image Pipelines
Source: arXiv:2112.09219 source file (2022-03-18)
Supplement: Supplementary file 1 [file supp_SO.tex]

The $S$ operator offers the functionality of a conventional (hardware) ISP pipeline using a sequence of cascaded sub-modules. In particular, the proposed $S$ operator consists of the following components: Bayer Demosaicking, color balancing, white balancing, contrast enhancement, Gamma adjustment, and colorspace conversion sub-modules. We provide the implementation details of each sub-module below:

% In this section, we provide more details regarding the $S$ operator of synthetic software ISP used in the proposed approach. Our pipeline consists of six main modules: Bayer Demosaicking module, Color Balance module, White Balance module, Contrast Improvement module, Gamma Adjustment module, and Colorspace Conversion module. Details of each module are illustrated below

\begin{enumerate}

\item{\textbf{Bayer Demosaicking}:} As discussed in the main manuscript, a color filter array (CFA) sits on a matrix of small potential wells. When light passes through the CFA layer, a mosaic pattern of the three stimulus RGB colors is generated, called RAW image. A Bayer pattern mosaic is the most commonly used one, alternating R-G-G-B $2 \times 2$ superpixels. To reconstruct trichromatic intensity values from a RAW image, a demosaicking algorithm is required. In our implementation, we use the DDFaPD demosaicking algorithm \cite{menon2006demosaicing} offered by the Python colour-demosaicing library.

% In a digital camera, a color filter array (CFA) is placed in front of an image sensor to record specific wavelengths of light on different photosite, resulting in the RAW captures with a Bayer mosaic (alternating R-G-G-B $2 \times 2$ color filter array). Trichromatic RGB values are reconstructed from RAW captures, for example by interpolation~\cite{zhang2011color}.  In our pipeline, we use DDFaPD demosaick algorithm \cite{menon2006demosaicing} implemented in Python colour-demosaicing library.
\vspace{2mm}
\item{\textbf{Color Balance }} The purpose of color balancing is to recover the color characteristics of the original scene. We achieve the color balancing by using the SimpleColorBalance \cite{limare2011simplest} algorithm, which is adopted from the OpenCV library. 

% The color balancing step aims to estimate the sensor's R, G, B color filter responses to lighting and adjust colors accordingly. We adopt the color balancing method from the OpenCV library, which implements the SimpleColorBalance \cite{limare2011simplest} algorithm based illumination estimation.

\vspace{2mm}
\item{\textbf{White Balance }:} We further adjust the color temperatures of RGB images with a white balance method to make the color look more natural. We use a white balancing method provided by the OpenCV library, mainly based on the White Patch algorithm and Gray World algorithm~\cite{rizzi2002color}.

\vspace{2mm}
\item{\textbf{Contrast Enhancement}} Contrast plays a critical role in separating the dark and bright areas of an image. An improvement in contrast increases this separation, making objects more distinguishable. In our pipeline, the Contrast Limited Adaptive Histogram Equalization(CLAHE) algorithm \cite{reza2004realization} is leveraged for contrast enhancement.

% Contrast improvement enhance the perceptibility of objects in the scene by improving the brightness difference between objects and their backgrounds. In our pipeline, we use the Contrast Limited Adaptive Histogram Equalization(CLAHE) algorithm \cite{reza2004realization}.

\vspace{2mm}
\item{\textbf{Gamma Adjustment}:} In this step, we use a non-linear Gamma correction function to adjust the image luminance (\ie, brightness level). In our pipeline, we use the OpenCV's gamma correction algorithm \cite{huang2012efficient}.

% Gamma curve is applied to the target image for modifying brightness and achieving more appealing details. In our pipeline, we use the default gamma correction algorithm \cite{huang2012efficient} from the OpenCV library.

\vspace{2mm}
\item{\textbf{Colorspace Conversion}:} Pixel values are converted to a specific colorspace (e.g., to sRGB) before compression (e.g. to jpg), storage, or further processing. 

\end{enumerate}

\noindent The $F$ operator is a small learned encoder-decoder network to map an RGB image to its intermediate RAW measurements. The details of network architecture are shown below in Table \ref{tab:RGB2RAW}

\begin{table}[]
    
	\centering
	\fontsize{9}{12}\selectfont   
	\vspace{-7mm}
	\caption{Architecture description of the $F$ Operator.}
	%\vspace{-2mm}
	\begin{tabular}{p{0.10\textwidth}p{0.28\textwidth}p{0.22\textwidth}
	p{0.22\textwidth}p{0.08\textwidth}}
		\toprule
% 		\cmidrule(lr){1-5}
		Layer & Type & In-Channel & Out-Channel & Kernel  \cr
		\cmidrule(lr){1-5}
		1st & Conv+Relu & 3 & 32 & 3$\times$3   \cr
		2nd & Conv+Relu & 32 & 64 & 3$\times$3   \cr
		3rd & Conv+Relu & 64 & 128 & 3$\times$3   \cr
		4th & UpConv+Relu & 128 & 64 & 3$\times$3   \cr
		5th & UpConv+Relu & 64 & 32 & 3$\times$3   \cr
		6th & UpConv+Sigmoid & 32 & 1 & 3$\times$3   \cr
		\bottomrule
	\end{tabular}\vspace{0cm}
	\label{tab:RGB2RAW}
	\vspace{-8mm}
\end{table}

% \begin{table}[]
% \vspace{-0mm}
% \begin{center}
% \begin{minipage}{0.9\linewidth}
%  \begin{adjustbox}{width=1\linewidth}
%  \fontsize{6}{9}\selectfont   
% 	\begin{tabular}{p{0.06\textwidth}p{0.2\textwidth}p{0.16\textwidth}
% 	p{0.16\textwidth}p{0.06\textwidth}}
% 		\toprule
% % 		\cmidrule(lr){1-5}
% 		Layer & Type & In-Channel & Out-Channel & Kernel  \cr
% 		\cmidrule(lr){1-5}
% 		1st & Conv+Relu & 3 & 32 & 3$\times$3   \cr
% 		2nd & Conv+Relu & 32 & 64 & 3$\times$3   \cr
% 		3rd & Conv+Relu & 64 & 128 & 3$\times$3   \cr
% 		4th & UpConv+Relu & 128 & 64 & 3$\times$3   \cr
% 		5th & UpConv+Relu & 64 & 32 & 3$\times$3   \cr
% 		6th & UpConv+Sigmoid & 32 & 1 & 3$\times$3   \cr
% 		\bottomrule
% 	\end{tabular}\vspace{0cm}
% \end{adjustbox}
% \end{minipage}
% \hfill
% \begin{minipage}{0.08\linewidth}
% %\vspace{3mm}
% \captionsetup{font=footnotesize,labelfont=footnotesize}
% \caption{
% {\textbf{Architecture description of the $F$ Operator}
% % : The $F$ operator is a small learned encoder-decoder network to map an RGB image to its intermediate RAW measurements.
% }
% }
% \label{tab:RGB2RAW}
% \end{minipage}
% \end{center}
% \vspace{-10mm}
% \end{table}
