# Supplementary material for: All You Need is RAW: Defending Against Adversarial Attacks with Camera Image Pipelines
Source: arXiv:2112.09219 source file (2022-03-18)
Supplement: Supplementary file 2 [file supp_attack.tex]

In this section, we provide formal definitions for the attack algorithms which are used for validation of the proposed defense method. 
\vspace{2mm}

\begin{enumerate}

\item{\textbf{FSGM:}} The FSGM~\cite{goodfellow2015explaining} is an attack method that, for each pixel, determines in which direction the pixel intensity should be moved according to the gradient of the loss function. Mathematically, the adversarial perturbation $\delta$ is defined by FGSM as:
% method designs the adversarial pattern by exploiting the gradient of the input image. Specifically, it determines the direction to modify each pixel value based on the gradient with respect to the loss function. Mathematically, given a clean input image x and corresponding ground truth label y, the attack method generate the adversarial perturbation $\delta$ by:

\begin{align*}
	\delta = \epsilon \cdot \text{sign}(\nabla_{x} L(x,y)),
\end{align*}
where $\epsilon$ is the maximum perturbation allowed for an attack, which is commonly sufficiently small for undetectable; $x$ and $y$ are a benign image and the corresponding ground truth label, respectively.
\vspace{2mm}

\item{\textbf{BIM:}} The BIM~\cite{kurakin2017adversarial} attack is an enhanced version of FGSM. Instead of taking one single step of size $\epsilon$, it iteratively searches for an optimal perturbation with multiple smaller steps $\alpha$. Then, the obtained perturbation is clipped by the predefined $\epsilon$. Formally, BIM is defined as
% attack improves FSGM by iteratively finding the optimal perturbation within the $\epsilon$ neighborhood of the input image.Specifically, given a clean input image x and corresponding ground truth label y. With the initial $x_0 = x$, the method iteratively find $x_i$ by

\begin{align*}
	x_i = \text{clip}_{\epsilon,x} (x_{i-1} + \alpha \cdot \text{sign}(\nabla_{x} L(x,y)) ),
\end{align*}
where $x_0 = x$. The number of iteration used is a hyperparameter, and more iterations typically lead to a stronger attack. 
\vspace{2mm}

\item{\textbf{PGD:}} Similar to the BIM attack, the PGD~\cite{madry2019deep} attack interatively optimzes the adversarial examples generated. With the initial $x_0 = x$, the method iteratively find $x_i$ by:

\begin{equation}
x^{i}=\Pi_{x+S}(x^{i-1}+\alpha\cdot \text{sign}(\nabla_x L(f_{\theta}(x^{i-1}),y))) ,
\end{equation}
where $\Pi_{x+S}$ denotes projecting perturbations into the set $S$. We refer the reader to \cite{madry2019deep} for additional details. The scalar $\alpha$ is the step size used in each iteration and $\epsilon$ denotes the maximum perturbation allowed. 
%\bd{Bo: not very clear to me}%

 \vspace{2mm}
 
\item{\textbf{DeepFool:}} Similar to BIM and PGD, the DeepFool~\cite{moosavidezfooli2016deepfool} attack generates adversarial perturbations iteratively, intending to obtain the perturbation with minimal distortion. Specifically, it finds the closest decision boundary by multiple linearizations of the classifier and then generates the perturbations based on the decision boundary.

\vspace{2mm}

\item{\textbf{C\&W:} The C\&W~\cite{carlini2017evaluating} attack is an optimization-based attack method, which generates the adversarial perturbations by solving the following problem

% The CW~\cite{carlini2017evaluating} attack is an optimization-based attack method. Given a clean input image x and corresponding ground truth label y, the attack algorithm finds the perturbation $\delta$ by:

\begin{align}
	& \min \ \ \ \ \ \ ||\delta||_p + c \cdot f(x+\delta) \nonumber\\ 
	& s.t.  \ \ \ \ \ \  x+\delta \in [0, 1]^n
\end{align}
\noindent where $f$ is a objective function that is designed to mislead the example $x$ to be misclassified; $||\cdot||_p$ denotes $l_p$ norm; and $c$ is a constant, estimated by binary search. 

\vspace{2mm}
\item{\textbf{NewtonFool:}} NewtonFool \cite{jang2017objective} attack is essentially a variant of DeepFool attack. In contrast to DeepFool generating perturbations based on linearization approximation, the NewtonFool is based on nonlinear constraints, allowing for a significantly faster generation of adversarial patterns. Hence, with the same time budget, more iterations can be performed, resulting in stronger attacks.

% NewtonFool~\cite{jang2017objective} attack is essentially a variant of DeepFool attack, which can generate even stronger adversarial patterns. Similar to DeepFool, it aims to find a strong adversarial example in the minimum neighborhood of input image through an iterative process. It differs from DeepFool that Newton’s method for solving nonlinear constraints. This practice allows for a significantly faster generation of adversarial patterns. With the same time constraints budget, more iteration can be performed, resulting in stronger attack.

\vspace{2mm}
\item{\textbf{DAG:}}}
The DAG~\cite{xie2017adversarial} attack is designed to attack semantic segmentation and object detection models. Essentially, it is similar to optimization-based classification attacks, generating adversarial perturbation by solving the following problem:
\begin{equation}
\label{eq:DAG}
    \forall n, {\arg\max_c\left\{f_c\!\left(\mathbf{X}+\mathbf{r},t_n\right)\right\}}\neq{l_n},
\end{equation}
where $X$ is an image which contains $N$ recognition targets ${\mathcal{T}}={\left\{t_1,t_2,\ldots,t_N\right\}}$; ${\mathcal{L}}={\left\{l_1,l_2,\ldots,l_n\right\}}$ is the ground-truth class labels of ${\mathcal{T}}$, \ie, $l_n$ is the ground-truth label of $t_n$; ${\mathbf{f}\!\left(\mathbf{X},t_n\right)}\in{\mathbb{R}^C}$
denote the classification score vector on the $n$-th recognition target; $\mathbf{r}$ denotes an adversarial perturbation to be estimated.

The form of ${\mathcal{T}}$ is defined based on a specific task. For the image classification task, ${\mathcal{T}}$ only contains one element, \ie, the entire image. ${\mathcal{T}}$ becomes all pixels for semantic segmentation tasks, while it becomes all proposals for object detection tasks.

\vspace{1mm}
Intuitively, the goal of the Eq.~\ref{eq:DAG} is to make the predictions of all targets incorrect by estimating an adversarial perturbation $\mathbf{r}$. In doing so, adversarial labels ${\mathcal{L}'}={\left\{l'_1,l'_2,\ldots,l'_n\right\}}\quad \forall i, l_i \neq l'_i$ are required, which are generated by randomly sampling from other incorrect classes.  Under this setting, the loss function covering all targets can be written as
\begin{equation}
\label{Eqn:LossFunction}
{L\!\left(\mathbf{X},\mathcal{T},\mathcal{L},\mathcal{L}'\right)}=
    {{\sum_{n=1}^N}\left[{f}_{l_n}\!\left(\mathbf{X},t_n\right)-{f}_{l_n'}\!\left(\mathbf{X},t_n\right)\right]}.
\end{equation}
Minimizing $L$ can be achieved by making every target an incorrect prediction, \ie, suppressing the confidence of the original correct class $f_{l_n}\!\left(\mathbf{X}+\mathrm{r},t_n\right)$,
while increasing  the confidence of desired (adversarial) incorrect class $f_{l'_n}\!\left(\mathbf{X}+\mathrm{r},t_n\right)$).

\end{enumerate}
