# Supplementary material for: All You Need is RAW: Defending Against Adversarial Attacks with Camera Image Pipelines
Source: arXiv:2112.09219 source file (2022-03-18)
Supplement: Supplementary file 3 [file supp_supper_white.tex]

\begin{table*}[h]
	% \begin{center}
		\vspace{-2mm}
		\begin{minipage}{0.71\linewidth}
			\begin{adjustbox}{width=1.4\linewidth}
				{\small
					\addtolength{\tabcolsep}{0pt}
					% \begin{tabular}{|l|c|c|c|c|c|c|c|c|c|}
					\begin{tabular}{l|ccccccccccc}
						\hline
						\hline
						 & \multicolumn{2}{c}{Super-FSGM} & \multicolumn{2}{c}{Super-PGD} & \multicolumn{2}{c}{Super-BIM} & \multicolumn{2}{c}{Super-DeepFool} & \multicolumn{2}{c}{Super-C\&W}  & Super-NewtonFool\\
						 & $2/255\uparrow$ & $4/255\uparrow$ &$2/255\uparrow$ & $4/255\uparrow$ & $2/255\uparrow$ & $4/255\uparrow$ & $L_{\infty}\uparrow$ & $L_{2}\uparrow$ & $L_{\infty}\uparrow$ & $L_{2}\uparrow$  &  $L_{\infty}\uparrow$
						 \\ 
						 \hline
						% \hline
						ComDefend\cite{jia2019comdefend} & 7.43 & 5.12&	1.33 & 0.80 &	1.54 &  0.82  &	1.83 & 1.70 &	2.47 & 1.02 &	0.45
								\\			
						Proposed method w/ $G$ only  & 11.97 & 7.82&	3.68 & 1.83 &	4.02 &  2.35  &	3.27 & 2.11 &	4.93 & 1.36 &	0.83
								\\									
						% \hline
						Proposed Method   & \textbf{62.88} & \textbf{55.25}  & \textbf{65.05}  & \textbf{63.97} &	\textbf{64.49} & \textbf{60.56} &	\textbf{68.62} & \textbf{59.93} &	\textbf{68.74} & \textbf{65.13}  &	\textbf{38.41}
						\\
						\hline
						\hline
						  
					\end{tabular}\\
				}
			\end{adjustbox}
		\end{minipage}
		\vspace{2mm}
		 \large{ \caption{We evaluate the defense performance against a super-white attack setting, where we assume the preprocessing model is exposed and the adversary can calculate the gradient for the differentiable part of the preprocessing model to construct stronger adversarial attacks. In such a setting, the differentiable preprocessing module (\ie, ComDefend and $G$ only) fail while our method does not collapse, demonstrating the benefit of exploiting the conventional ISP operator $S$ in our method.}  \label{tbl:super-white}}
	% \end{center}
	\vspace{-8mm}
\end{table*}

We conduct a super-white attack experiment to provide insights into the benefits of the proposed non-differentiable $S$ operator. A white-box setting means the attack methods have full access to a target model, including network architecture,  learned weights, and even training data, yet not to the preprocessing module used to transform input. In contrast, in the super-white box attack setting, both preprocessing modules and target models are exposed, allowing the adversary to calculate the gradient for adversarial attacks. In Table~\ref{tbl:super-white}, we demonstrate the defense performances of three competing approaches on the ImageNet in Top-1 accuracy under the super-white box attack setting. We see that the defense methods with differentiable preprocessing modules (\ie, ComDefend and the proposed method with $G$ only) cannot function effectively under the super-white box attack setting. The attack only impacts the proposed method marginally, validating the benefit of the non-differentiable $S$ operator. 
