# Supplementary material for: All You Need is RAW: Defending Against Adversarial Attacks with Camera Image Pipelines
Source: arXiv:2112.09219 source file (2022-03-18)
Supplement: Supplementary file 4 [file supp_Qualitative_result.tex]

\begin{figure*}[]
	\centering
	\resizebox{\linewidth}{!}{
	
	\begin{tabular}{ccccccccccc}
	
		\includegraphics[width=0.35\columnwidth, trim={0cm 0cm 0cm 0cm},clip]{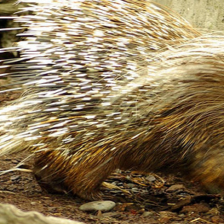}&
		\includegraphics[width=.35\columnwidth, trim={0cm 0cm 0cm 0cm},clip]{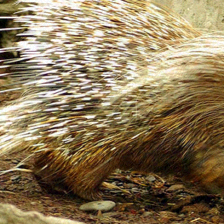}&
		\includegraphics[width=0.35\columnwidth, trim={0cm 0cm 0cm 0cm},clip]{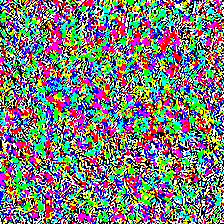}&
		\includegraphics[width=.35\columnwidth, trim={0cm 0cm 0cm 0cm},clip]{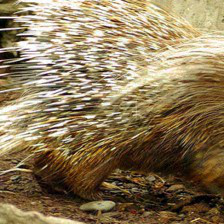} &	
		\includegraphics[width=.35\columnwidth, trim={0cm 0cm 0cm 0cm},clip]{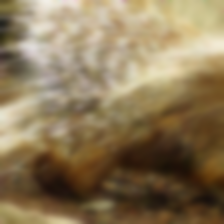} &
		\includegraphics[width=.35\columnwidth, trim={0cm 0cm 0cm 0cm},clip]{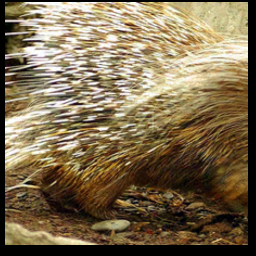} & 
		\includegraphics[width=.35\columnwidth, trim={0cm 0cm 0cm 0cm},clip]{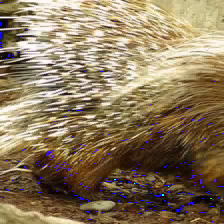} &
		\includegraphics[width=.35\columnwidth, trim={0cm 0cm 0cm 0cm},clip]{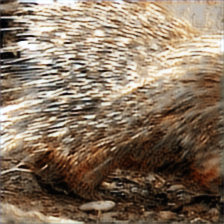} &	
		\includegraphics[width=.35\columnwidth, trim={0cm 0cm 0cm 0cm},clip]{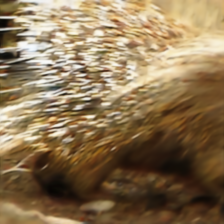}&
		\includegraphics[width=.35\columnwidth, trim={0cm 0cm 0cm 0cm},clip]{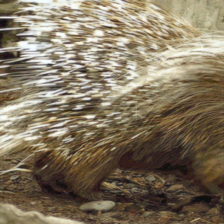} &
		\includegraphics[width=.35\columnwidth, trim={0cm 0cm 0cm 0cm},clip]{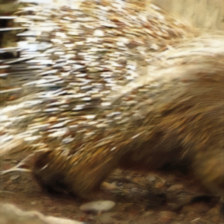} 		
		\\[.2cm]

		\includegraphics[width=0.35\columnwidth, trim={0cm 0cm 0cm 0cm},clip]{figs/results/visual_our_png/000031_original_images.png}&
		\includegraphics[width=.35\columnwidth, trim={0cm 0cm 0cm 0cm},clip]{figs/results/visual_our_png/000031_adv_images.png}&
		\includegraphics[width=0.35\columnwidth, trim={0cm 0cm 0cm 0cm},clip]{figs/results/visual_our_png/000031_perturbation.png}&
		\includegraphics[width=.35\columnwidth, trim={0cm 0cm 0cm 0cm},clip]{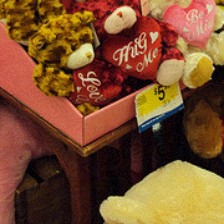} &	
		\includegraphics[width=.35\columnwidth, trim={0cm 0cm 0cm 0cm},clip]{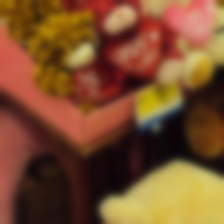} &
		\includegraphics[width=.35\columnwidth, trim={0cm 0cm 0cm 0cm},clip]{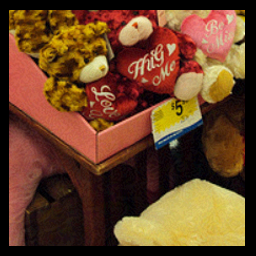} & 
		\includegraphics[width=.35\columnwidth, trim={0cm 0cm 0cm 0cm},clip]{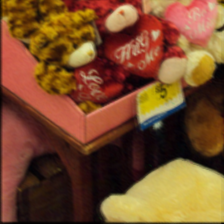} &
		\includegraphics[width=.35\columnwidth, trim={0cm 0cm 0cm 0cm},clip]{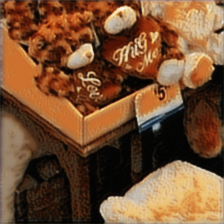} &	
		\includegraphics[width=.35\columnwidth, trim={0cm 0cm 0cm 0cm},clip]{figs/results/visual_our_png/000031_recons_deep_isp.png}&
		\includegraphics[width=.35\columnwidth, trim={0cm 0cm 0cm 0cm},clip]{figs/results/visual_our_png/000031_recons_isp.png} &
		\includegraphics[width=.35\columnwidth, trim={0cm 0cm 0cm 0cm},clip]{figs/results/visual_our_png/000031_recons_weighted.png} 	
		\\[.2cm]
		
		\includegraphics[width=0.35\columnwidth, trim={0cm 0cm 0cm 0cm},clip]{figs/results/visual_our_png/000081_original_images.png}&
		\includegraphics[width=.35\columnwidth, trim={0cm 0cm 0cm 0cm},clip]{figs/results/visual_our_png/000081_adv_images.png}&
		\includegraphics[width=0.35\columnwidth, trim={0cm 0cm 0cm 0cm},clip]{figs/results/visual_our_png/000081_perturbation.png}&
		\includegraphics[width=.35\columnwidth, trim={0cm 0cm 0cm 0cm},clip]{figs/results/visual_JPEG_png/000081_recons_weighted.png} &	
		\includegraphics[width=.35\columnwidth, trim={0cm 0cm 0cm 0cm},clip]{figs/results/visual_pixel_TVM_png/000081_recons_weighted.png} &
		\includegraphics[width=.35\columnwidth, trim={0cm 0cm 0cm 0cm},clip]{figs/results/visual_pixel_ResizePad_png/000081_recons_weighted.png} & 
		\includegraphics[width=.35\columnwidth, trim={0cm 0cm 0cm 0cm},clip]{figs/results/visual_pixel_deflection_png/000081_recons_weighted.png} &
		\includegraphics[width=.35\columnwidth, trim={0cm 0cm 0cm 0cm},clip]{figs/results/visual_comdefend_png/000081_recons_weighted.png} &	
		\includegraphics[width=.35\columnwidth, trim={0cm 0cm 0cm 0cm},clip]{figs/results/visual_our_png/000081_recons_deep_isp.png}&
		\includegraphics[width=.35\columnwidth, trim={0cm 0cm 0cm 0cm},clip]{figs/results/visual_our_png/000081_recons_isp.png} &
		\includegraphics[width=.35\columnwidth, trim={0cm 0cm 0cm 0cm},clip]{figs/results/visual_our_png/000081_recons_weighted.png} 	
		\\[.2cm]	
		
		\includegraphics[width=0.35\columnwidth, trim={0cm 0cm 0cm 0cm},clip]{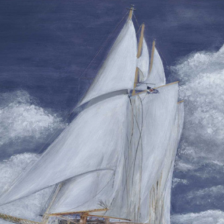}&
		\includegraphics[width=.35\columnwidth, trim={0cm 0cm 0cm 0cm},clip]{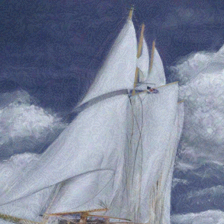}&
		\includegraphics[width=0.35\columnwidth, trim={0cm 0cm 0cm 0cm},clip]{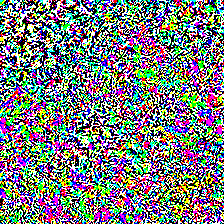}&
		\includegraphics[width=.35\columnwidth, trim={0cm 0cm 0cm 0cm},clip]{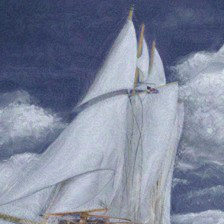} &
		\includegraphics[width=.35\columnwidth, trim={0cm 0cm 0cm 0cm},clip]{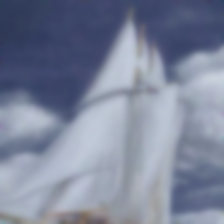} &
		\includegraphics[width=.35\columnwidth, trim={0cm 0cm 0cm 0cm},clip]{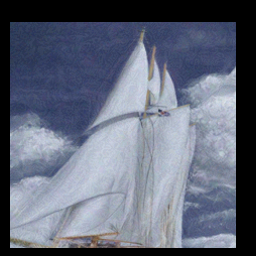} & 
		\includegraphics[width=.35\columnwidth, trim={0cm 0cm 0cm 0cm},clip]{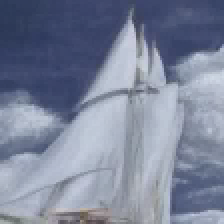} &
		\includegraphics[width=.35\columnwidth, trim={0cm 0cm 0cm 0cm},clip]{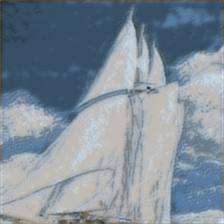} &	
		\includegraphics[width=.35\columnwidth, trim={0cm 0cm 0cm 0cm},clip]{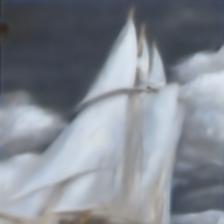}&
		\includegraphics[width=.35\columnwidth, trim={0cm 0cm 0cm 0cm},clip]{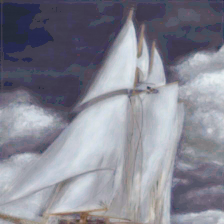} &
		\includegraphics[width=.35\columnwidth, trim={0cm 0cm 0cm 0cm},clip]{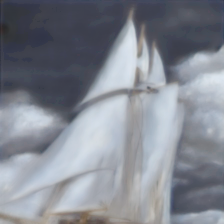} 	
		\\[.2cm]
		
		\includegraphics[width=0.35\columnwidth, trim={0cm 0cm 0cm 0cm},clip]{figs/results/visual_our_png/000085_original_images.png}&
		\includegraphics[width=.35\columnwidth, trim={0cm 0cm 0cm 0cm},clip]{figs/results/visual_our_png/000085_adv_images.png}&
		\includegraphics[width=0.35\columnwidth, trim={0cm 0cm 0cm 0cm},clip]{figs/results/visual_our_png/000085_perturbation.png}&
		\includegraphics[width=.35\columnwidth, trim={0cm 0cm 0cm 0cm},clip]{figs/results/visual_JPEG_png/000085_recons_weighted.png} &	
		\includegraphics[width=.35\columnwidth, trim={0cm 0cm 0cm 0cm},clip]{figs/results/visual_pixel_TVM_png/000085_recons_weighted.png} &
		\includegraphics[width=.35\columnwidth, trim={0cm 0cm 0cm 0cm},clip]{figs/results/visual_pixel_ResizePad_png/000085_recons_weighted.png} & 
		\includegraphics[width=.35\columnwidth, trim={0cm 0cm 0cm 0cm},clip]{figs/results/visual_pixel_deflection_png/000085_recons_weighted.png} &
		\includegraphics[width=.35\columnwidth, trim={0cm 0cm 0cm 0cm},clip]{figs/results/visual_comdefend_png/000085_recons_weighted.png} &	
		\includegraphics[width=.35\columnwidth, trim={0cm 0cm 0cm 0cm},clip]{figs/results/visual_our_png/000085_recons_deep_isp.png}&
		\includegraphics[width=.35\columnwidth, trim={0cm 0cm 0cm 0cm},clip]{figs/results/visual_our_png/000085_recons_isp.png} &
		\includegraphics[width=.35\columnwidth, trim={0cm 0cm 0cm 0cm},clip]{figs/results/visual_our_png/000085_recons_weighted.png} 	
		\\[.2cm]			

		\includegraphics[width=0.35\columnwidth, trim={0cm 0cm 0cm 0cm},clip]{figs/results/visual_our_png/000087_original_images.png}&
		\includegraphics[width=.35\columnwidth, trim={0cm 0cm 0cm 0cm},clip]{figs/results/visual_our_png/000087_adv_images.png}&
		\includegraphics[width=0.35\columnwidth, trim={0cm 0cm 0cm 0cm},clip]{figs/results/visual_our_png/000087_perturbation.png}&
		\includegraphics[width=.35\columnwidth, trim={0cm 0cm 0cm 0cm},clip]{figs/results/visual_JPEG_png/000087_recons_weighted.png} &	
		\includegraphics[width=.35\columnwidth, trim={0cm 0cm 0cm 0cm},clip]{figs/results/visual_pixel_TVM_png/000087_recons_weighted.png} &
		\includegraphics[width=.35\columnwidth, trim={0cm 0cm 0cm 0cm},clip]{figs/results/visual_pixel_ResizePad_png/000087_recons_weighted.png} & 
		\includegraphics[width=.35\columnwidth, trim={0cm 0cm 0cm 0cm},clip]{figs/results/visual_pixel_deflection_png/000087_recons_weighted.png} &
		\includegraphics[width=.35\columnwidth, trim={0cm 0cm 0cm 0cm},clip]{figs/results/visual_comdefend_png/000087_recons_weighted.png} &	
		\includegraphics[width=.35\columnwidth, trim={0cm 0cm 0cm 0cm},clip]{figs/results/visual_our_png/000087_recons_deep_isp.png}&
		\includegraphics[width=.35\columnwidth, trim={0cm 0cm 0cm 0cm},clip]{figs/results/visual_our_png/000087_recons_isp.png} &
		\includegraphics[width=.35\columnwidth, trim={0cm 0cm 0cm 0cm},clip]{figs/results/visual_our_png/000087_recons_weighted.png} 	
		\\[.2cm]	
		
		\includegraphics[width=0.35\columnwidth, trim={0cm 0cm 0cm 0cm},clip]{figs/results/visual_our_png/000065_original_images.png}&
		\includegraphics[width=.35\columnwidth, trim={0cm 0cm 0cm 0cm},clip]{figs/results/visual_our_png/000065_adv_images.png}&
		\includegraphics[width=0.35\columnwidth, trim={0cm 0cm 0cm 0cm},clip]{figs/results/visual_our_png/000065_perturbation.png}&
		\includegraphics[width=.35\columnwidth, trim={0cm 0cm 0cm 0cm},clip]{figs/results/visual_JPEG_png/000065_recons_weighted.png} &
		\includegraphics[width=.35\columnwidth, trim={0cm 0cm 0cm 0cm},clip]{figs/results/visual_pixel_TVM_png/000065_recons_weighted.png} &
		\includegraphics[width=.35\columnwidth, trim={0cm 0cm 0cm 0cm},clip]{figs/results/visual_pixel_ResizePad_png/000065_recons_weighted.png} & 
		\includegraphics[width=.35\columnwidth, trim={0cm 0cm 0cm 0cm},clip]{figs/results/visual_pixel_deflection_png/000065_recons_weighted.png} &
		\includegraphics[width=.35\columnwidth, trim={0cm 0cm 0cm 0cm},clip]{figs/results/visual_comdefend_png/000065_recons_weighted.png} &	
		\includegraphics[width=.35\columnwidth, trim={0cm 0cm 0cm 0cm},clip]{figs/results/visual_our_png/000065_recons_deep_isp.png}&
		\includegraphics[width=.35\columnwidth, trim={0cm 0cm 0cm 0cm},clip]{figs/results/visual_our_png/000065_recons_isp.png} &
		\includegraphics[width=.35\columnwidth, trim={0cm 0cm 0cm 0cm},clip]{figs/results/visual_our_png/000065_recons_weighted.png} 	
		\\[.2cm]
		
		\includegraphics[width=0.35\columnwidth, trim={0cm 0cm 0cm 0cm},clip]{figs/results/visual_our_png/000030_original_images.png}&
		\includegraphics[width=.35\columnwidth, trim={0cm 0cm 0cm 0cm},clip]{figs/results/visual_our_png/000030_adv_images.png}&
		\includegraphics[width=0.35\columnwidth, trim={0cm 0cm 0cm 0cm},clip]{figs/results/visual_our_png/000030_perturbation.png}&
		\includegraphics[width=.35\columnwidth, trim={0cm 0cm 0cm 0cm},clip]{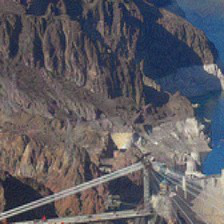} &
		\includegraphics[width=.35\columnwidth, trim={0cm 0cm 0cm 0cm},clip]{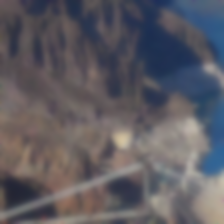} &
		\includegraphics[width=.35\columnwidth, trim={0cm 0cm 0cm 0cm},clip]{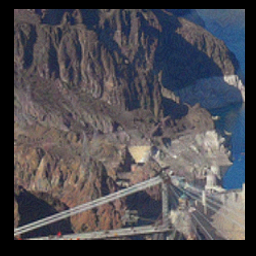} & 
		\includegraphics[width=.35\columnwidth, trim={0cm 0cm 0cm 0cm},clip]{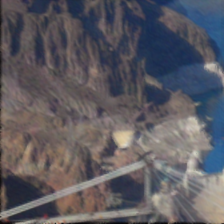} &
		\includegraphics[width=.35\columnwidth, trim={0cm 0cm 0cm 0cm},clip]{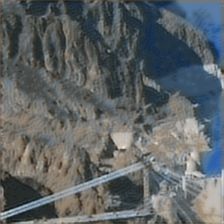} &	
		\includegraphics[width=.35\columnwidth, trim={0cm 0cm 0cm 0cm},clip]{figs/results/visual_our_png/000030_recons_deep_isp.png}&
		\includegraphics[width=.35\columnwidth, trim={0cm 0cm 0cm 0cm},clip]{figs/results/visual_our_png/000030_recons_isp.png} &
		\includegraphics[width=.35\columnwidth, trim={0cm 0cm 0cm 0cm},clip]{figs/results/visual_our_png/000030_recons_weighted.png} 	
		\\[.2cm]	

		\includegraphics[width=0.35\columnwidth, trim={0cm 0cm 0cm 0cm},clip]{figs/results/visual_our_png/000036_original_images.png}&
		\includegraphics[width=.35\columnwidth, trim={0cm 0cm 0cm 0cm},clip]{figs/results/visual_our_png/000036_adv_images.png}&
		\includegraphics[width=0.35\columnwidth, trim={0cm 0cm 0cm 0cm},clip]{figs/results/visual_our_png/000036_perturbation.png}&
		\includegraphics[width=.35\columnwidth, trim={0cm 0cm 0cm 0cm},clip]{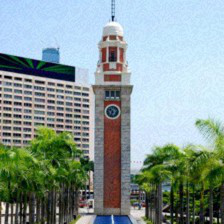} &
		\includegraphics[width=.35\columnwidth, trim={0cm 0cm 0cm 0cm},clip]{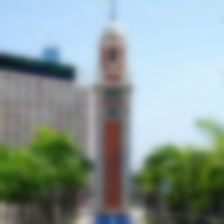} &
		\includegraphics[width=.35\columnwidth, trim={0cm 0cm 0cm 0cm},clip]{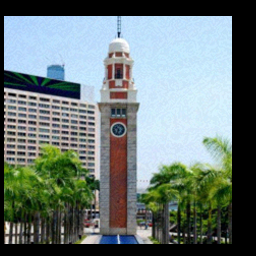} & 
		\includegraphics[width=.35\columnwidth, trim={0cm 0cm 0cm 0cm},clip]{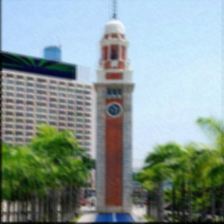} &
		\includegraphics[width=.35\columnwidth, trim={0cm 0cm 0cm 0cm},clip]{figs/results/visual_comdefend_png/000036_recons_weighted.png} &	
		\includegraphics[width=.35\columnwidth, trim={0cm 0cm 0cm 0cm},clip]{figs/results/visual_our_png/000036_recons_deep_isp.png}&
		\includegraphics[width=.35\columnwidth, trim={0cm 0cm 0cm 0cm},clip]{figs/results/visual_our_png/000036_recons_isp.png} &
		\includegraphics[width=.35\columnwidth, trim={0cm 0cm 0cm 0cm},clip]{figs/results/visual_our_png/000036_recons_weighted.png} 	
		\\[.2cm]	
		
		\includegraphics[width=0.35\columnwidth, trim={0cm 0cm 0cm 0cm},clip]{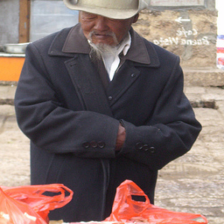}&
		\includegraphics[width=.35\columnwidth, trim={0cm 0cm 0cm 0cm},clip]{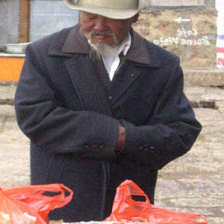}&
		\includegraphics[width=0.35\columnwidth, trim={0cm 0cm 0cm 0cm},clip]{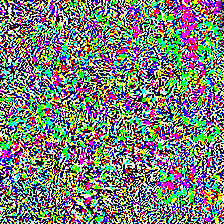}&
		\includegraphics[width=.35\columnwidth, trim={0cm 0cm 0cm 0cm},clip]{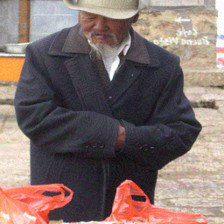} &
		\includegraphics[width=.35\columnwidth, trim={0cm 0cm 0cm 0cm},clip]{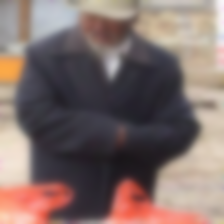} &
		\includegraphics[width=.35\columnwidth, trim={0cm 0cm 0cm 0cm},clip]{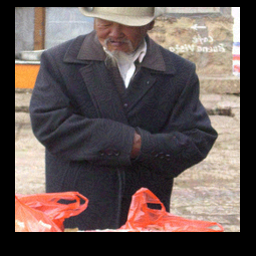} & 
		\includegraphics[width=.35\columnwidth, trim={0cm 0cm 0cm 0cm},clip]{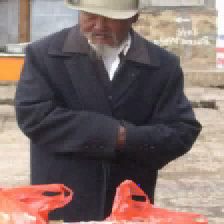} &
		\includegraphics[width=.35\columnwidth, trim={0cm 0cm 0cm 0cm},clip]{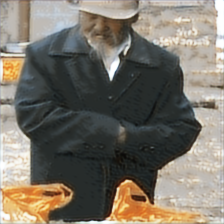} &	
		\includegraphics[width=.35\columnwidth, trim={0cm 0cm 0cm 0cm},clip]{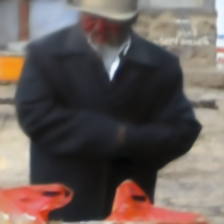}&
		\includegraphics[width=.35\columnwidth, trim={0cm 0cm 0cm 0cm},clip]{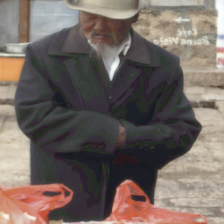} &
		\includegraphics[width=.35\columnwidth, trim={0cm 0cm 0cm 0cm},clip]{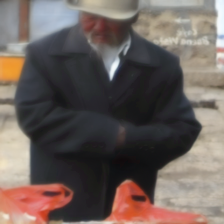} 		
		\\[.2cm]		
		
		\includegraphics[width=0.35\columnwidth, trim={0cm 0cm 0cm 0cm},clip]{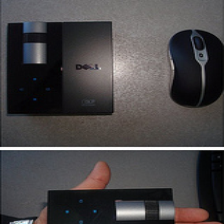}&
		\includegraphics[width=.35\columnwidth, trim={0cm 0cm 0cm 0cm},clip]{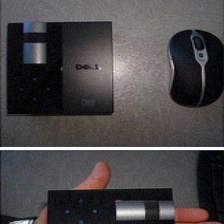}&
		\includegraphics[width=0.35\columnwidth, trim={0cm 0cm 0cm 0cm},clip]{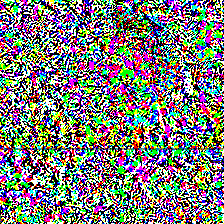}&
		\includegraphics[width=.35\columnwidth, trim={0cm 0cm 0cm 0cm},clip]{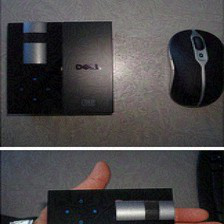} &
		\includegraphics[width=.35\columnwidth, trim={0cm 0cm 0cm 0cm},clip]{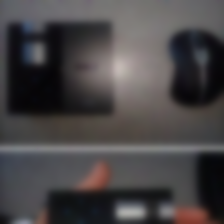} &
		\includegraphics[width=.35\columnwidth, trim={0cm 0cm 0cm 0cm},clip]{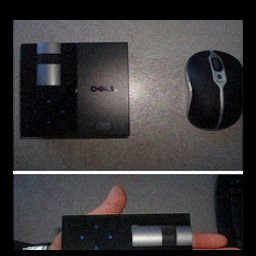} & 
		\includegraphics[width=.35\columnwidth, trim={0cm 0cm 0cm 0cm},clip]{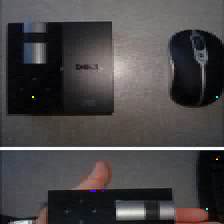} &
		\includegraphics[width=.35\columnwidth, trim={0cm 0cm 0cm 0cm},clip]{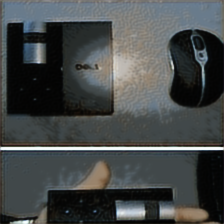} &	
		\includegraphics[width=.35\columnwidth, trim={0cm 0cm 0cm 0cm},clip]{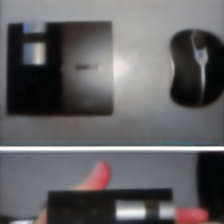}&
		\includegraphics[width=.35\columnwidth, trim={0cm 0cm 0cm 0cm},clip]{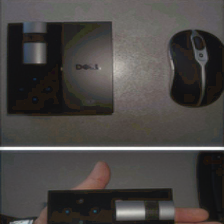} &
		\includegraphics[width=.35\columnwidth, trim={0cm 0cm 0cm 0cm},clip]{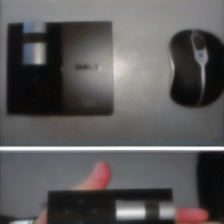} 	
		\\[.2cm]			

		\includegraphics[width=0.35\columnwidth, trim={0cm 0cm 0cm 0cm},clip]{figs/results/visual_our_png/000051_original_images.png}&
		\includegraphics[width=.35\columnwidth, trim={0cm 0cm 0cm 0cm},clip]{figs/results/visual_our_png/000051_adv_images.png}&
		\includegraphics[width=0.35\columnwidth, trim={0cm 0cm 0cm 0cm},clip]{figs/results/visual_our_png/000051_perturbation.png}&
		\includegraphics[width=.35\columnwidth, trim={0cm 0cm 0cm 0cm},clip]{figs/results/visual_JPEG_png/000051_recons_weighted.png} &
		\includegraphics[width=.35\columnwidth, trim={0cm 0cm 0cm 0cm},clip]{figs/results/visual_pixel_TVM_png/000051_recons_weighted.png} &
		\includegraphics[width=.35\columnwidth, trim={0cm 0cm 0cm 0cm},clip]{figs/results/visual_pixel_ResizePad_png/000051_recons_weighted.png} & 
		\includegraphics[width=.35\columnwidth, trim={0cm 0cm 0cm 0cm},clip]{figs/results/visual_pixel_deflection_png/000051_recons_weighted.png} &
		\includegraphics[width=.35\columnwidth, trim={0cm 0cm 0cm 0cm},clip]{figs/results/visual_comdefend_png/000051_recons_weighted.png} &	
		\includegraphics[width=.35\columnwidth, trim={0cm 0cm 0cm 0cm},clip]{figs/results/visual_our_png/000051_recons_deep_isp.png}&
		\includegraphics[width=.35\columnwidth, trim={0cm 0cm 0cm 0cm},clip]{figs/results/visual_our_png/000051_recons_isp.png} &
		\includegraphics[width=.35\columnwidth, trim={0cm 0cm 0cm 0cm},clip]{figs/results/visual_our_png/000051_recons_weighted.png} 	
		\\[.2cm]	

		\includegraphics[width=0.35\columnwidth, trim={0cm 0cm 0cm 0cm},clip]{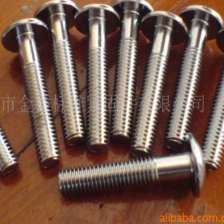}&
		\includegraphics[width=.35\columnwidth, trim={0cm 0cm 0cm 0cm},clip]{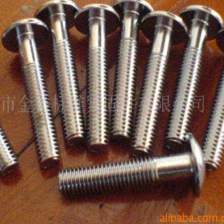}&
		\includegraphics[width=0.35\columnwidth, trim={0cm 0cm 0cm 0cm},clip]{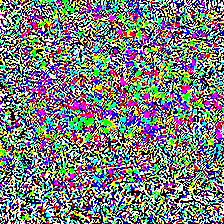}&
		\includegraphics[width=.35\columnwidth, trim={0cm 0cm 0cm 0cm},clip]{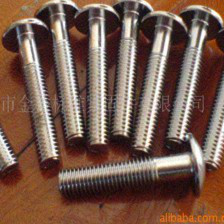} &
		\includegraphics[width=.35\columnwidth, trim={0cm 0cm 0cm 0cm},clip]{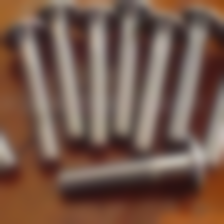} &
		\includegraphics[width=.35\columnwidth, trim={0cm 0cm 0cm 0cm},clip]{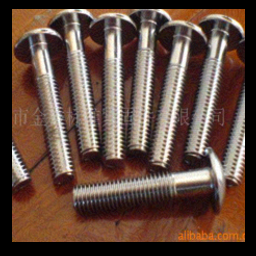} & 
		\includegraphics[width=.35\columnwidth, trim={0cm 0cm 0cm 0cm},clip]{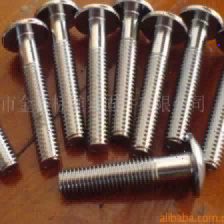} &
		\includegraphics[width=.35\columnwidth, trim={0cm 0cm 0cm 0cm},clip]{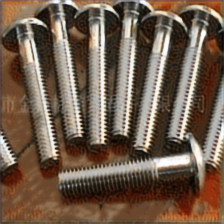} &	
		\includegraphics[width=.35\columnwidth, trim={0cm 0cm 0cm 0cm},clip]{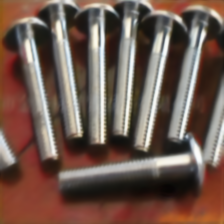}&
		\includegraphics[width=.35\columnwidth, trim={0cm 0cm 0cm 0cm},clip]{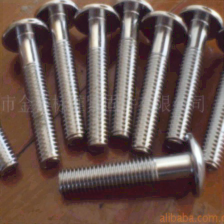} &
		\includegraphics[width=.35\columnwidth, trim={0cm 0cm 0cm 0cm},clip]{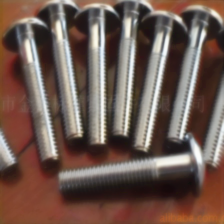} 	
		\\[.2cm]

		\centering
		{ \huge{Clean Image}}&
		{ \huge{Adversarial Image}}&
		{ \huge{Perturbation}}&		
		{ \huge{JPEG-Defense\cite{JPEG_eval}}} &
		{ \huge{TVM\cite{guo2017countering} }} &
		{ \huge{Resizing \& Padding\cite{xie2017mitigating} }} &
		{ \huge{Pixel-Deflection\cite{prakash2018deflecting}}} &
		{ \huge{ComDefend\cite{jia2019comdefend}}} & 
		{ \huge{Operator $G$}}&
		{ \huge{Operator $S$}} &
		{ \huge{Proposed Method}} 		
		\\		
	\end{tabular} 
	}
	\vspace{-2mm}
    \caption{\footnotesize{Qualitative comparison of the proposed method along with both $G$ and $S$ operators against state-of-the-art defense methods on the ImageNet dataset, see text.}}
    \label{fig:more_qualitative} 
    % \caption{\textbf{Qualitative Examples.} We show qualitative examples of baseline defense methods and the proposed method, including the operator outputs of $G$ and $S$. }
    \vspace{-2mm}
\end{figure*}

In this section, we provide additional qualitative results from the proposed methods and state-of-the-art defense baselines. For input-transformation-based adversarial defense methods, a balance between transformation fidelity and adversarial patterns removal is essential. A higher transformation fidelity indicates more details of the original image are kept, including adversarial patterns. In contrast, radical pattern removal could result in a severe loss of detail. This balance is achieved by a simple weighted sum between the $G$ and $S$ operator in our method. The $S$ operator is designed for faithfully reconstructing high-frequency details, while the $G$ operator is trained to mitigate adversarial patterns. As shown in Figure \ref{fig:more_qualitative}, our approach offers better transformation fidelity than Comdefend, TVM, Pixel Deflection, and Resizing \& Padding methods. Even though the JPEG-Defense method keeps more high-frequency details than the ones offered by our approach, it suffers from removing adversarial patterns, resulting in the worst performance among all compared methods.

% In this section, we show more qualitative results from the proposed methods and state-of-the-art defense baselines in figure \ref{fig:more_qualitative}. For the adversarial defense method based on input transformation, a good balance between transformation fidelity and adversarial patterns removal is required. A high fidelity means the transformed image keeps the same details as the input image. However,  a 100\% fidelity would lead to 0\% defense accuracy, as all adversarial patterns are kept. On the contrary, radical pattern mitigation would remove most of the adversarial patterns, but at the same time, may result in a severe loss of details that help the decision-making of downstream models.  Thus, a good balance between transformation fidelity and adversarial patterns removal is required. In our method, the G operator learns to mitigate the adversarial pattern, while the S operator can faithfully reconstruct high-frequency details.  Combining them in a weighted sum manner allows us to achieve such a good balance. As the figure \ref{fig:more_qualitative} shows, compared to the baseline method, we achieve better transformation fidelity than Comdefend, TVM, Pixel Deflection, Resizing \& Padding. Meanwhile, JPEG-Defense keeps too many details from the input image, resulting in limited removal adversarial pattern and thus the worst performance among all the methods.
